# Supplementary material for: Angular velocity of gravitational radiation from precessing binaries and the corotating frame
Source: arXiv:1302.2919 ancillary file (2013-04-10)
Supplement: Supplementary file 1 [file Documentation.pdf]

Note that most of the documentation for various objects and functions is accessible via Doxygen, by opening `html/index.html` in the code directory. Almost all of that documentation is also available through Python's built-in `help` function described below.

This IPython notebook should be opened with the command

```
ipython notebook Documentation.ipynb --pylab
```

If you have not opened it in this way, or have opened a different file, you are missing out...

## Sec. I: Introduction

This IPython notebook contains examples for the GWFrames code provided with the paper "Angular velocity of gravitational radiation from precessing binaries and the corotating frame" by Michael Boyle. This notebook roughly mirrors the paper itself, providing examples of code relevant to each of the sections. The notebook works basically like a Mathematica notebook. In particular, this is connected to a live Python session. You should be able to put your cursor into a code cell and press Shift+Enter to evaluate the cell, just as in Mathematica.

### Sec. I B: Overview of this code

This code is written primarily in C++, and can be used directly through that interface, as demonstrated in the subdirectory `C++Example`. All classes and functions are in the `GWFrames` namespace. However, a more interactive interface is provided via Python as the `GWFrames` module. (This is implemented through SWIG, using the file `GWFrames.i`.)

If you have not yet compiled the module, run `make` in the code directory. Then, to get started, load this module by evaluating the cell below. If you see any errors, the module did not install properly. If everything is working properly, you should see no output. For more details, see the `README` file.

```
In [1]: import GWFrames

# While we're at it, set up plots
import GWFrames.plot
from mpl_toolkits.mplot3d import Axes3D # For 3D plots
mpl.rcParams['figure.figsize'] = 8,6 # Set default figure size (in inches)
%config InlineBackend.figure_format='svg' # If plotting inline, use SVG
```

IPython provides tab completion, which helps you see your options. In the cell below, put your cursor after the '.', and press tab. You should see a list of the various objects and functions provided by the `GWFrames` module.

```
In [ ]: GWFrames.
```

The primary objects provided by this module are the `Waveform`, `PNWaveform`, and `Quaternion` objects. We can call the default constructors for these objects as follows:

```
In [2]: W_NR = GWFrames.Waveform()
W_PN = GWFrames.PNWaveform()
Q = GWFrames.Quaternion()
```

Each of these objects has various member functions that can act on them. Place your cursor at the end of any line below and press tab to see a list of possibilities. The `PNWaveform` object is a subclass of the `Waveform` object, so it has all the same methods plus a few more.

```
In [ ]: W_NR.
        W_PN.
        Q.
```

IPython also provides a useful help feature, which shows built-in documentation. Just put a question mark after any object or class to see its documentation. For example, evaluate the following cell to see what a `PNWaveform` is and how to call its constructors:

```
In [3]: GWFrames.PNWaveform?
```

We find that we can construct a `PNWaveform` object as

```
In [4]: # First, define the parameters for convenience
        m1 = 6.
        chi1Mag = 0.9
        vartheta1 = 2.
        varphi1 = 0.25
        chi1 = [chi1Mag*sin(vartheta1)*cos(varphi1), chi1Mag*sin(vartheta1)*sin(varphi1), chi1Mag*cos(vartheta1)]
        m2 = 1.
        chi2Mag = 0.3
        vartheta2 = 2.4
        varphi2 = 2.9
        chi2 = [chi2Mag*sin(vartheta2)*cos(varphi2), chi2Mag*sin(vartheta2)*sin(varphi2), chi2Mag*cos(vartheta2)]
        Omega0 = 0.02

        # Now create the PNWaveform object
        W_PN = GWFrames.PNWaveform((m1-m2)/(m1+m2), chi1, chi2, Omega0);

        # And transform to the inertial frame
        W_PN.TransformToInertialFrame();
```

We can also read in a waveform object from a data file. The data are assumed to be in columns, where the first column is the time and successive columns are the magnitude and phase of the modes. Alternatively, it is possible to read data with columns of the real and imaginary parts of the modes by switching "MagArg" to "ReIm" below. The modes are assumed to be in the order  $(2, -2), (2, -1), \dots$

If this is not the case, they must be reordered manually.

```
In [5]: # W_NR = GWFrames.Waveform("/path/to/data/rhOverM.dat", "MagArg")
```

If you have started this notebook with the `--pylab` option, you can plot the data. (Note that this plot may appear in a separate window that does not pop up in front of the browser on some systems. Look for it behind your browser.)

```
In [6]: i22 = W_PN.FindModeIndex(2,2) # Find the index of the (2,2) mode
plot(W_PN.T(), W_PN.Re(i22)); plot(W_PN.T(), W_PN.Im(i22)); # Plot the real and imaginary parts o.
xlabel(r"${t-t_{\mathrm{merger}}}/M$");
ylabel(r"Strain");
```

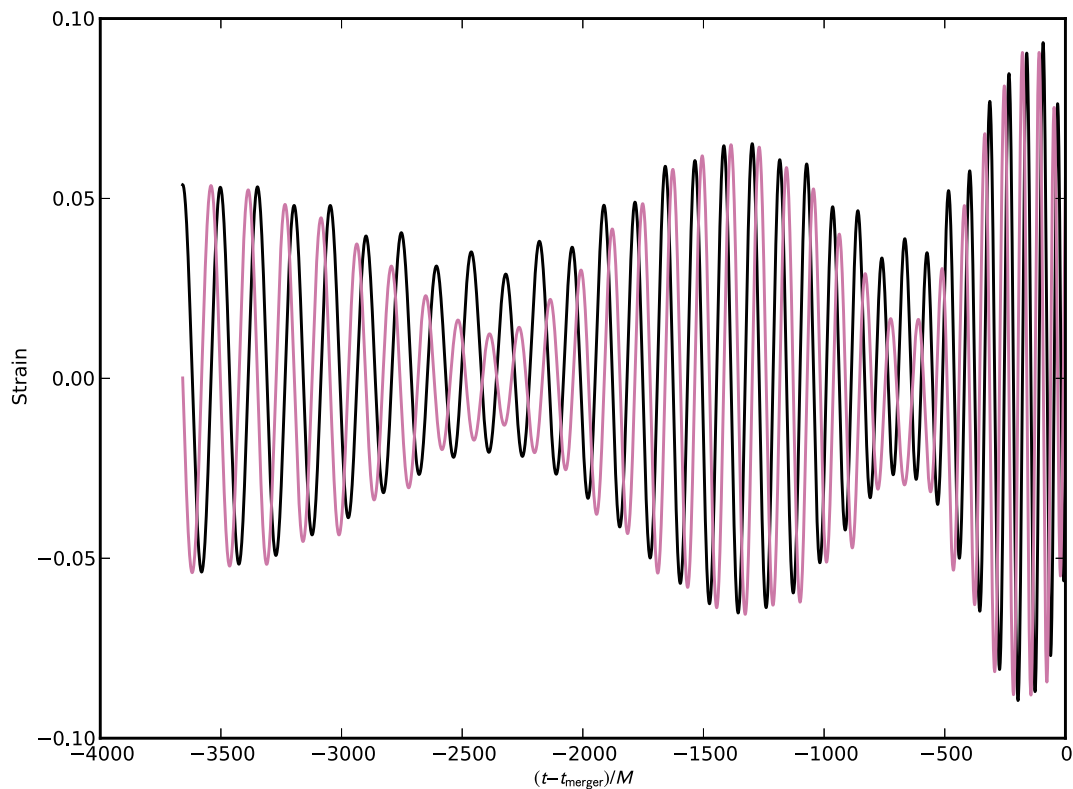

### Sec. I C: Quaternion notation

Quaternion objects can be created (to make up a couple random examples) as

```
In [7]: Q1 = GWFrames.Quaternion(3,1,4,1)
Q2 = GWFrames.Quaternion(5.9,2.6,5.3,5.8)
```

We can take the conjugate and the norm:

```
In [8]: print( Q1.conjugate() )
print( Q1.abs() )

[3, -1, -4, -1]
5.19615242271
```

We can construct a vector and a rotor, and then rotate the vector. This constructs  $\hat{z}$ , then rotates it by an angle  $\pi/2$  about the  $x$  axis, which gives us  $-\hat{y}$  (up to machine precision):

```
In [9]: z = GWFrames.Quaternion([0,0,1])
R = GWFrames.exp( (pi/2) * GWFrames.Quaternion([1,0,0]) / 2)
R*z*R.conjugate()
```

```
Out[9]: Quaternion(0.0, 0.0, -1.0, 2.220446049250313e-16)
```

Note that we have used the quaternion exponential function to define  $R$  above. We also have the logarithm function. Here, we take the logarithm of  $R$  to find a vector with  $\pi/4$  in the  $x$  component:

```
In [10]: GWFrames.log(R)
```

```
Out[10]: Quaternion(0.0, 0.7853981633974482, 0.0,
0.0)
```

## Sec. II: Angular velocity of a waveform

The angular velocity of a waveform can be obtained directly from either a `Waveform` object or a `PNWaveform` object. Assuming you have constructed the `w_PN` object above, you can run this

```
In [11]: # Get the angular-velocity vector of W_PN, using all ell modes
# by default (PNWaveforms have ell ranging from 2 to 8)
AV_PN = array(W_PN.AngularVelocityVector())

# Now plot it in 3D
fig = plt.figure()
ax = fig.gca(projection='3d')
ax.plot(AV_PN[:,0], AV_PN[:,1], AV_PN[:,2], label=r"$\vec{\omega}$")
ax.legend()
fig.tight_layout(pad=0.1)
plt.show()
```

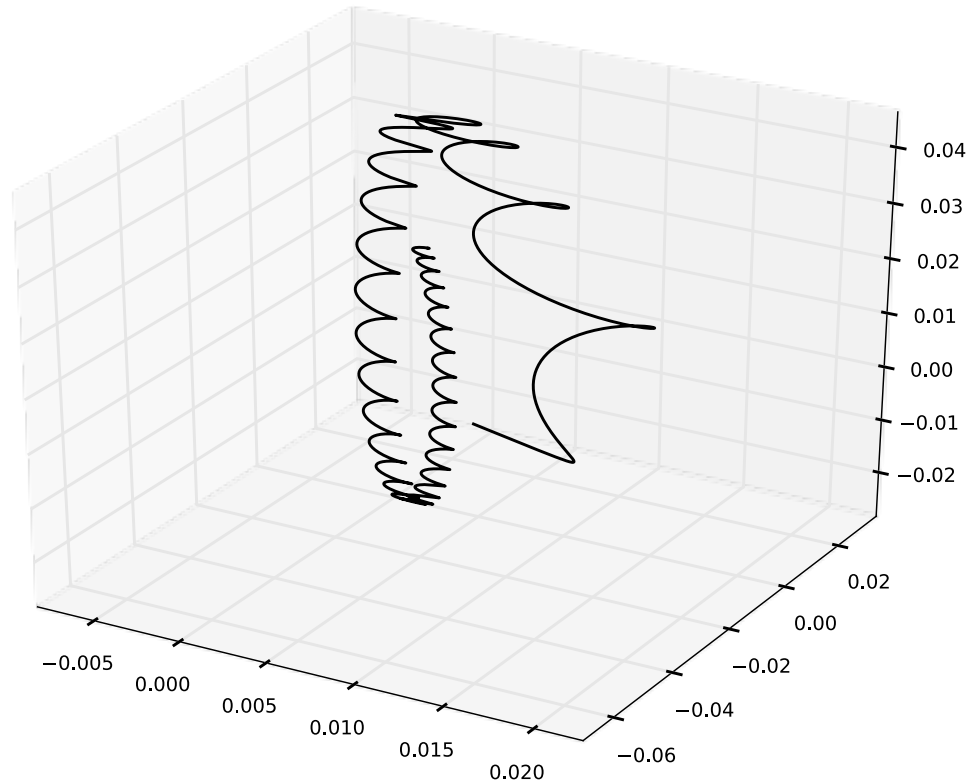

## Sec. III: Solving the inverse problem

A `PNWaveform` object records the orbital and precessional angular velocities of the binary. We can look at these and compare to the "PN-equivalent" orbital and total angular velocities that are obtained from the waveform data alone. The following reproduces Fig. 1 from the paper. The next cell below will demonstrate the related `PNEquivalentOrbitalAV` and `PNEquivalentPrecessionalAV` methods, which are available for both `PNWaveform` and `Waveform` objects.

```

In [12]: # Compute the various vectors
OmegaHat_orb = array(W_PN.OmegaHat_orb())
VHat_h = array(W_PN.OShaughnessyEtAlVector())
Omega_tot = array(W_PN.Omega_tot())
omega = array(W_PN.AngularVelocityVector())

# Plot the orbital AV vectors
fig = plt.figure()
ax = fig.gca(projection='3d')
ax.plot(OmegaHat_orb[:,0], OmegaHat_orb[:,1], OmegaHat_orb[:,2], lw=1, label=r"$\hat{\Omega}_{\rm orb}$")
ax.plot(VHat_h[:,0], VHat_h[:,1], VHat_h[:,2], ls='--', lw=2, label=r"$\hat{V}_h$")
ax.legend()
fig.tight_layout(pad=0.1)
plt.show()

# Plot the total AV vectors
fig = plt.figure()
ax = fig.gca(projection='3d')
ax.plot(Omega_tot[:,0], Omega_tot[:,1], Omega_tot[:,2], lw=1, label=r"$\vec{\Omega}_{\rm tot}$")
ax.plot(omega[:,0], omega[:,1], omega[:,2], ls='--', lw=2, label=r"$\vec{\omega}$")
ax.legend()
fig.tight_layout(pad=0.1)
plt.show()

```

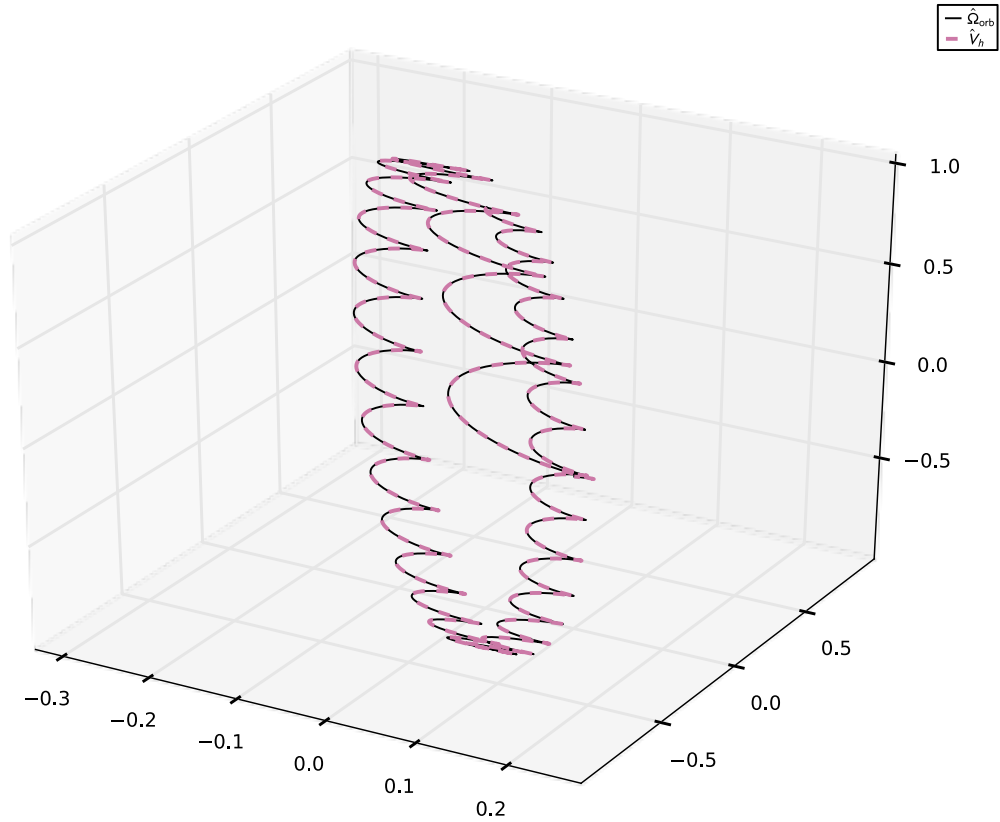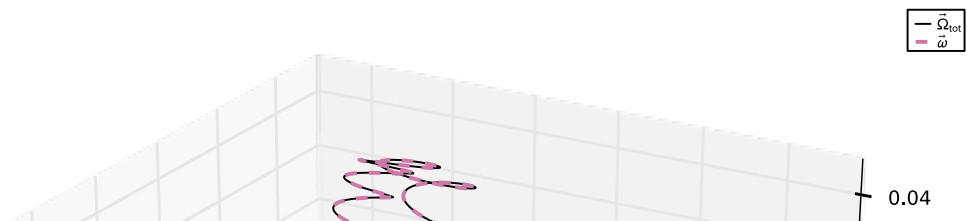

```

In [13]: # Compute the various vectors
Omega_orb = array(W_PN.Omega_orb())
OrbitalAV_equiv = array(W_PN.PNEquivalentOrbitalAV())
Omega_prec = array(W_PN.Omega_prec())
PrecessionalAV_equiv = array(W_PN.PNEquivalentPrecessionalAV())

# Plot the orbital AV vectors
fig = plt.figure()
ax = fig.gca(projection='3d')
ax.plot(Omega_orb[:,0], Omega_orb[:,1], Omega_orb[:,2], lw=1, label=r"$\vec{\Omega}_{\mathrm{orb}}$")
ax.plot(OrbitalAV_equiv[:,0], OrbitalAV_equiv[:,1], OrbitalAV_equiv[:,2], ls='--', lw=2,
        label=r"$(\hat{V}_h \cdot \vec{\omega}) \hat{V}_h$")
ax.legend()
fig.tight_layout(pad=0.1)
plt.show()

# Plot the precessional AV vectors
fig = plt.figure()
ax = fig.gca(projection='3d')
ax.plot(Omega_prec[:,0], Omega_prec[:,1], Omega_prec[:,2], lw=1, label=r"$\vec{\Omega}_{\mathrm{prec}}$")
ax.plot(PrecessionalAV_equiv[:,0], PrecessionalAV_equiv[:,1], PrecessionalAV_equiv[:,2], ls='--',
        label=r"$\vec{\omega} - (\hat{V}_h \cdot \vec{\omega}) \hat{V}_h$")
ax.legend()
fig.tight_layout(pad=0.1)
plt.show()

```

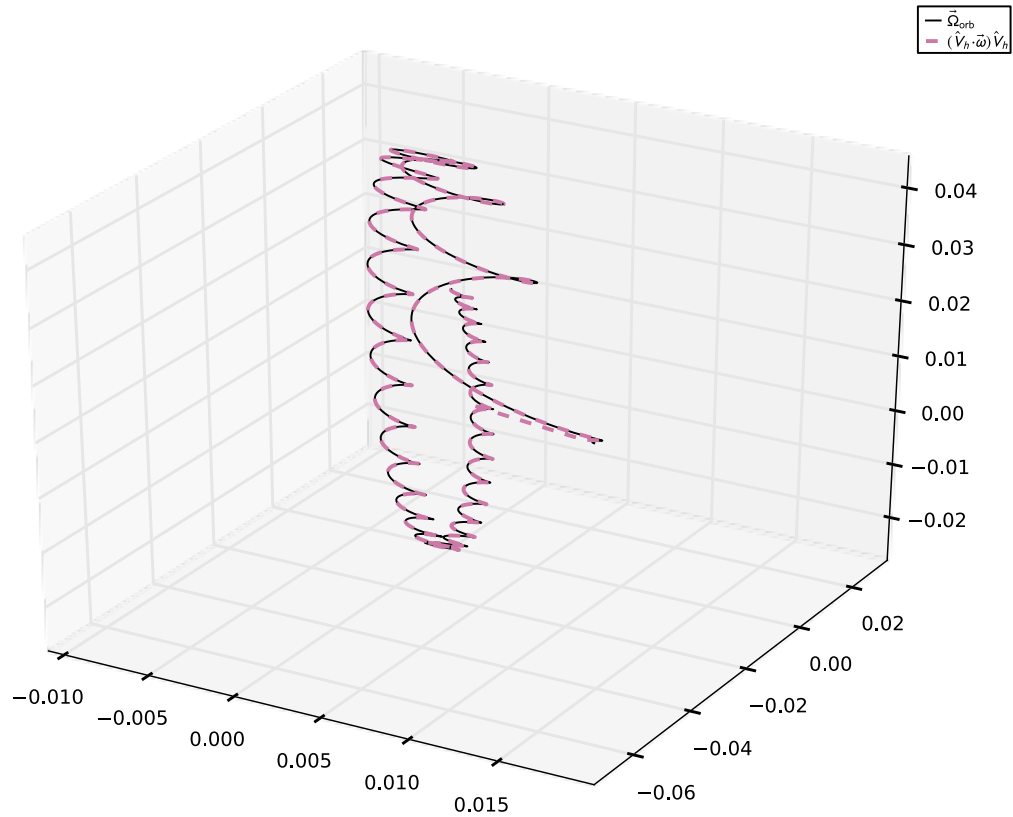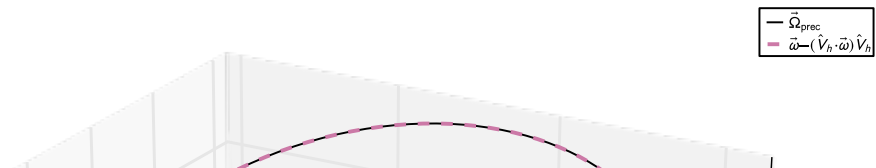

## Sec. IV: The corotating frame

### Sec. IV A: Finding the corotating frame

Given an array of quaternions representing the angular-velocity vector as a function of time, we can derive the appropriate corotating frame. [Note that Sec. IV B demonstrates a function that computes this frame and transforms the waveform in one easy step.]

```
In [14]: # Measure the angular-velocity vector from the waveform
AV_PN = array(W_PN.AngularVelocityVector())

# Get an array of quaternions representing the corotating frame
R_corot = GWFrames.FrameFromAngularVelocity(GWFrames.Quaternions(AV_PN), W_PN.T())
```

The system starts out mostly rotating about the  $z$  axis, due to the orbital motion, but also precessing a little. The frame at the third time step has been rotated about an axis that is mostly parallel to  $z$ , but has a slight  $x$  component:

```
In [15]: Rotor = R_corot[2]
Angle = Rotor.angle()
Axis = array(Rotor.log().vec())*(2/Angle)
Time = W_PN.T(2)-W_PN.T(0)
print("Time = {t}M after beginning\nRotor = {r}\nAxis = {ax}\nAngle = {a}".
      format(r=Rotor, ax=Axis.tolist(), a=Angle, t=Time))

print("\nNote that we started the system at an angular frequency of {O}, and the system
has gone through an angle {a:.4} after time {t:.4}, which makes sense.".format(O=Omega0, a=Angle, t=Time))

Time = 0.21648187372M after beginning
Rotor = [0.99999763120407, 0.0002259688109875, 2.5767373833356e-11, 0.0021648381794948]
Axis = [0.10381734921533284, 1.1838361391242967e-08, 0.9945963794433909]
Angle = 0.00435320283402

Note that we started the system at an angular frequency of 0.02, and the system
has gone through an angle 0.004353 after time 0.2165, which makes sense.
```

### Sec. IV B: Gravitational waveforms in the corotating frame

Now, rather than explicitly asking for the angular velocity, then the corotating frame, and then transforming the waveform, we can do it all in one go with the simple `TransformTo` methods:



```

In [16]: # Make copies to transform. Because Python makes copies by reference,
# to make a real copy, we need to use the copy constructor:
W_PN_Corot = GWFrames.PNWaveform(W_PN)
W_PN_Aligned = GWFrames.PNWaveform(W_PN)

# Now, transform the copies to the corotating frame and aligned frame
W_PN_Corot.TransformToCorotatingFrame()
W_PN_Aligned.TransformToOShaughnessyEtAlFrame()

# And plot the waveforms in the different frames
ell=2
ModeIndices = [W_PN.FindModeIndex(ell,m) for m in range(-ell,ell+1)]
plt.figure(1)
plt.subplot(321)
for ModeIndex in ModeIndices: plt.plot(W_PN.T(), W_PN.Abs(ModeIndex))
ylabel(r"$|r\, h^{2,m}/M\,|$");
plt.subplot(322)
for ModeIndex in ModeIndices: plt.plot(W_PN.T(), W_PN.ArgUnwrapped(ModeIndex))
ylabel(r"$\phi^{2,m}$ (radians)");
plt.subplot(323)
for ModeIndex in ModeIndices: plt.plot(W_PN_Aligned.T(), W_PN_Aligned.Abs(ModeIndex))
ylabel(r"$|r\, h^{2,m}/M\,|$");
plt.subplot(324)
for ModeIndex in ModeIndices: plt.plot(W_PN_Aligned.T(), W_PN_Aligned.ArgUnwrapped(ModeIndex))
ylabel(r"$\phi^{2,m}$ (radians)");
plt.subplot(325)
for ModeIndex in ModeIndices: plt.plot(W_PN_Corot.T(), W_PN_Corot.Abs(ModeIndex))
ylabel(r"$|r\, h^{2,m}/M\,|$");
xlabel(r"$ (t-t_{\mathrm{merger}})/M$");
plt.subplot(326)
for ModeIndex in ModeIndices: plt.plot(W_PN_Corot.T(), W_PN_Corot.ArgUnwrapped(ModeIndex))
ylabel(r"$\phi^{2,m}$ (radians)");
xlabel(r"$ (t-t_{\mathrm{merger}})/M$");

```

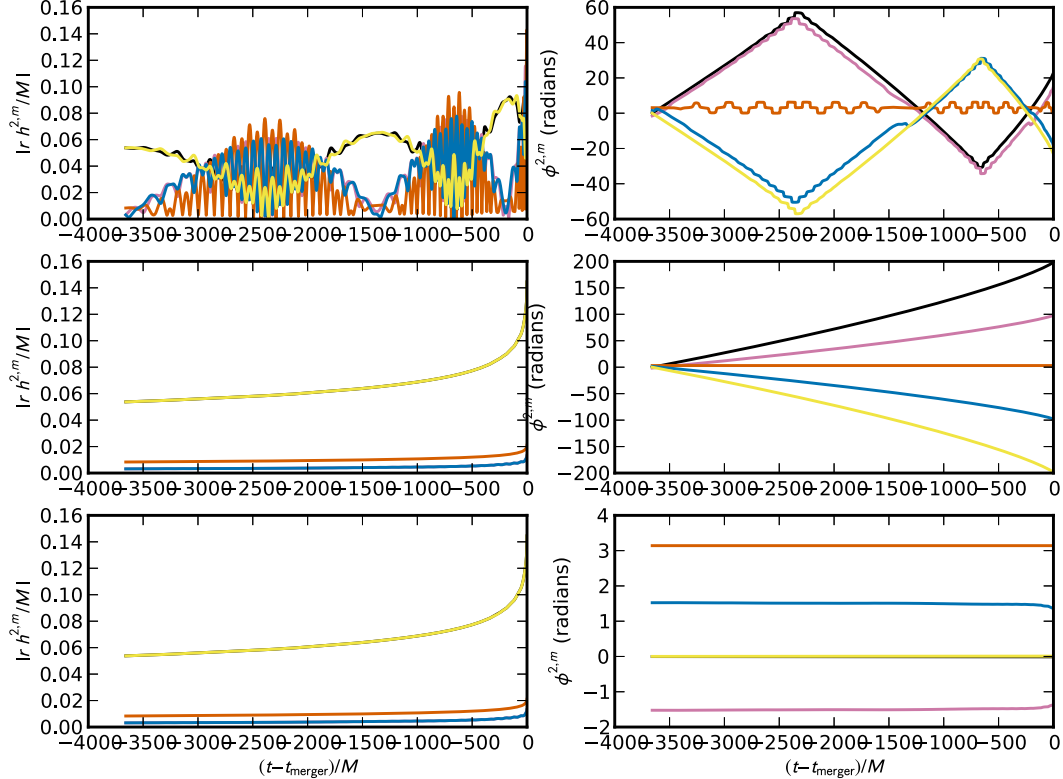

## Sec. IV C: Comparison, alignment, and hybridization

We can also compare, align, and hybridize any two waveform objects. (Extrapolation is beyond the scope of this documentation, though several functions provided here can certainly be useful.) First, we construct two objects that should be very nearly the same.

```
In [32]: # Create the waveforms in their inertial frames
W_A = GWFrames.PNWaveform(W_PN);
W_B = GWFrames.PNWaveform((m1-m2)/(m1+m2), chi1, chi2, 0.999*Omega0);
W_B.TransformToInertialFrame();
```

Note that the spin directions are defined at two slightly different frequencies, so these waveforms do not describe the same physics. But we choose to compare them just so there is some nontrivial difference for demonstration purposes. We can construct a new `Waveform` object, which records the difference between the modes and the frames. In this case, the frames are the same (because they are inertial), but the modes are very different:

```
In [33]: W_diff = W_A.Compare(W_B)
figure()
for m in range(-2,2+1) : plot(W_diff.T(), W_diff.Re(W_diff.FindModeIndex(2,m)), label=r'$m={0}$'.
ylabel(r"$\Delta \text{Re}\{r^2 \dot{h}^{2,m}/M\}$");
xlabel(r"$t-t_{\text{merger}}/M$");
legend();
```

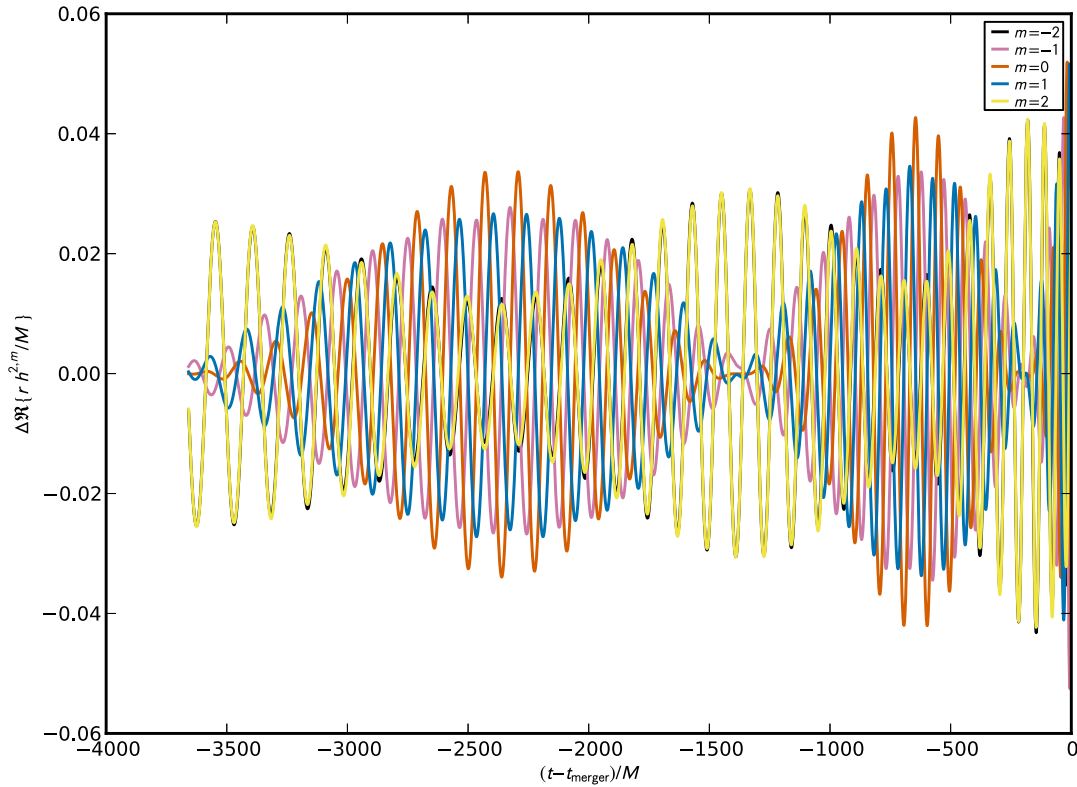

Now, we can also align the two waveforms. Because these systems are highly precessing, their angular frequencies are not monotonic -- and in particular, are not invertible everywhere. But we are hoping to align them by comparing angular frequencies, so we have to find a suitable time for which the angular frequency is invertible. We will be leaving `w_B` fixed, so we look for an angular frequency in that waveform that only occurs at one time. We plot the quantity below, and find that  $(t - t_{\text{merger}})/M = -3075$ , for example, is a suitable value.

```
In [34]: W_A_AVMag = [GWFrames.abs(a) for a in W_A.AngularVelocityVector()]
W_B_AVMag = [GWFrames.abs(a) for a in W_B.AngularVelocityVector()]
semilogy(W_A.T()[10:], W_A_AVMag[10:], label="W_A");
semilogy(W_B.T()[10:], W_B_AVMag[10:], label="W_B");
ylabel(r"$|\vec{\omega}|$, $\text{\vec{\omega}}$, |$");
xlabel(r"$-(t-t_{\mathrm{merger}})/M$");
legend();
```

Out[34]: <matplotlib.legend.Legend at 0x10a92add0>

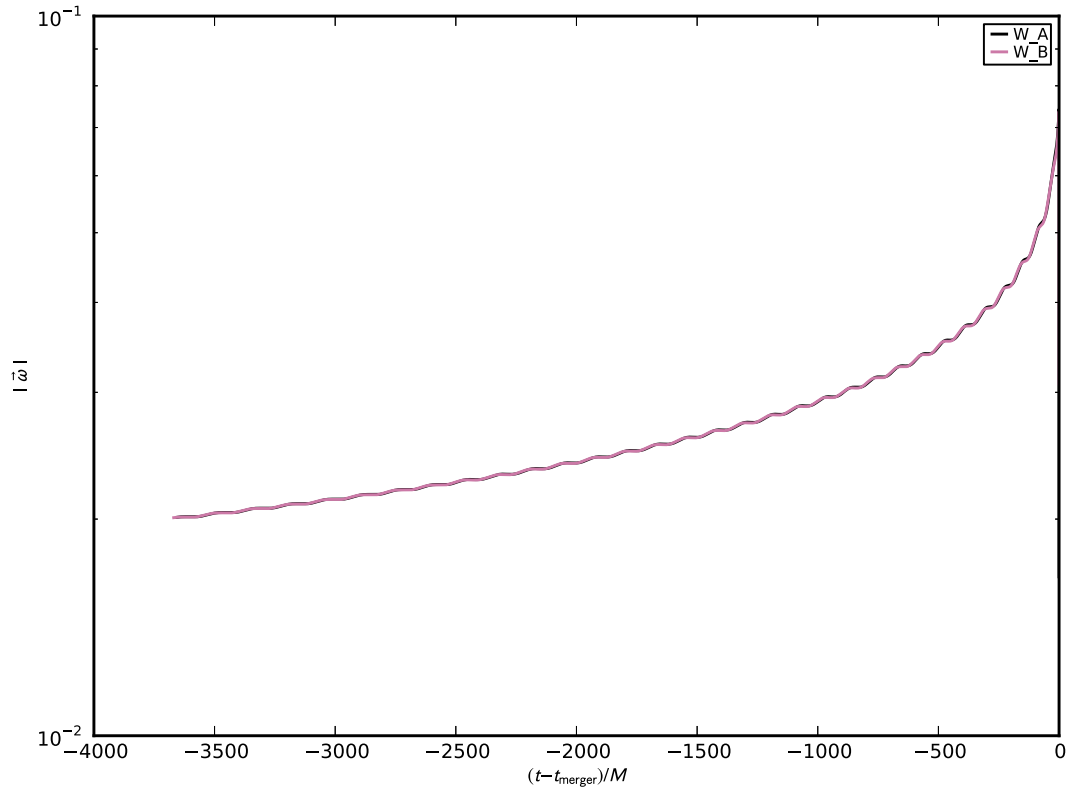

Then, we can align the two Waveforms by ensuring that they have the same  $|\vec{\omega}|$  at that moment:

```

In [35]: # Do the alignment
t_fid = -3075
W_A.AlignTime(W_B, t_fid);

# Now, plot the angular velocities, zooming in near -3075
W_A_AVMag = [GWFrames.abs(a) for a in W_A.AngularVelocityVector()]
plot(W_B.T()[10:], W_B_AVMag[10:], label="W_B");
plot(W_A.T()[10:], W_A_AVMag[10:], label="W_A");
xlim([-3500, -2500]);
ylim([2e-2, 2.3e-2]);
ylabel(r"$|\vec{\omega}|$");
xlabel(r"$\mathbf{(t-t_{\mathrm{merger}})}/M$");
legend();

```

Out[35]: <matplotlib.legend.Legend at 0x109a8f310>

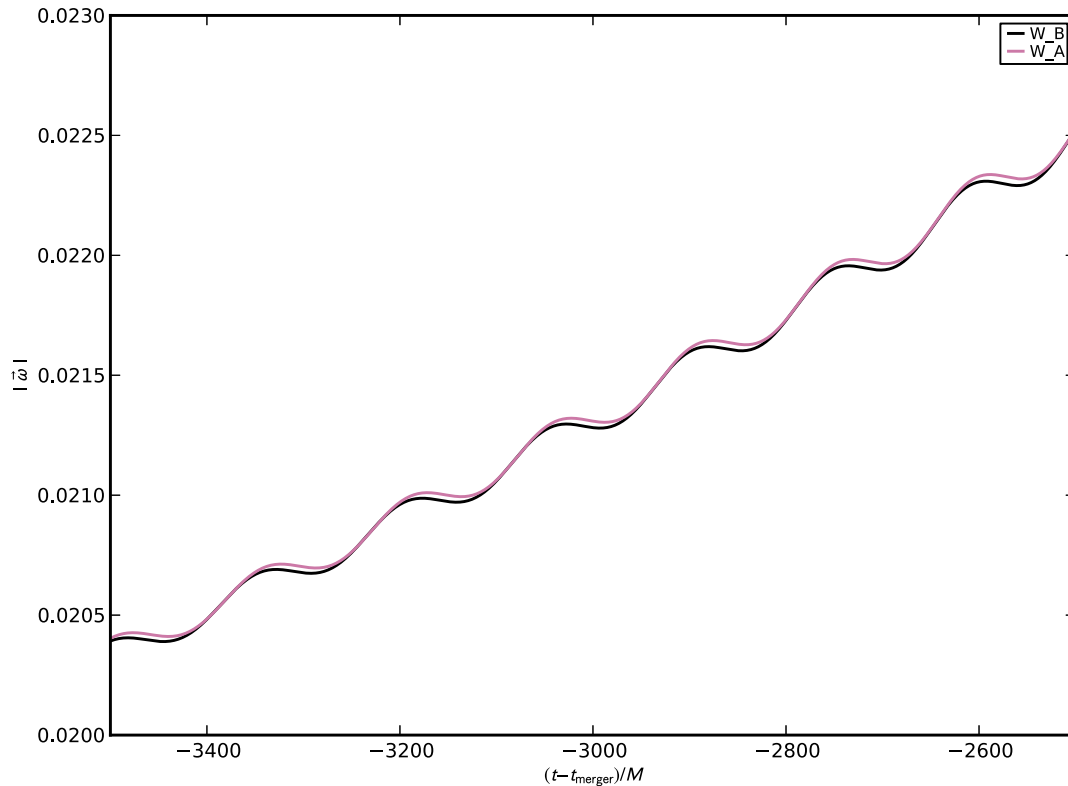

Note that the curves above intersect at -3075.

However, this only aligns the times at that instant. We may also want to align the Waveforms. To do this, we move into a physically meaningful frame (the corotating frame), ensuring that the modes are truly aligned to that frame, and then ensure that the frames are the same:

```

In [36]: # Transform to corotating frames
W_A.TransformToCorotatingFrame();
W_B.TransformToCorotatingFrame();

# Ensure that the modes and frames in each Waveform are aligned to each other
W_A.AlignDecompositionFrameToModes(t_fid)
W_B.AlignDecompositionFrameToModes(t_fid)

# Now simply align the frames to each other
W_A.AlignFrame(W_B, t_fid);

# Show the differences
W_diff = W_A.Compare(W_B)
figure()
for m in range(-2,2+1) : plot(W_diff.T(), W_diff.Re(W_diff.FindModeIndex(2,m)), label=r'$m={0}$'.
ylabel(r"$\Delta \text{Re}\{r\, h^{2,m}/M\, \}$");
xlabel(r"$ (t-t_{\mathrm{merger}})/M$");
legend();
figure()
plot(W_diff.T(), [r.angle() for r in W_diff.Frame()]);
ylabel(r"$\Phi_{\Delta}$ (radians)");
xlabel(r"$ (t-t_{\mathrm{merger}})/M$");

```

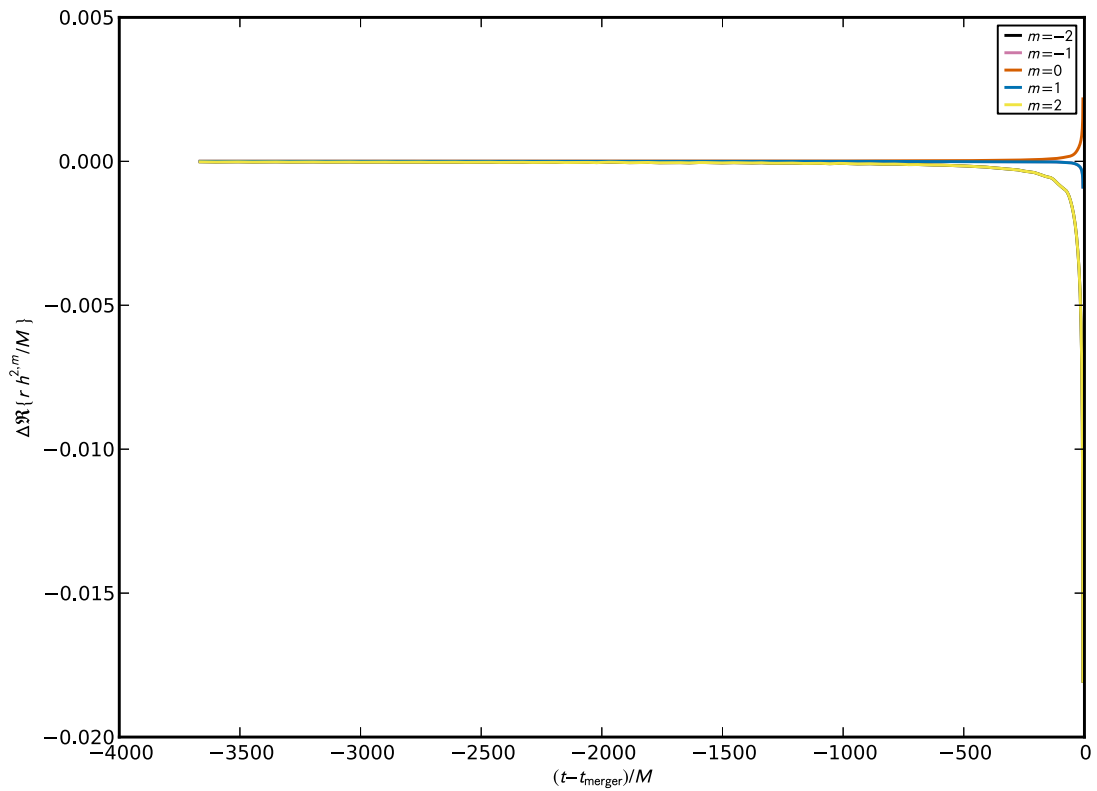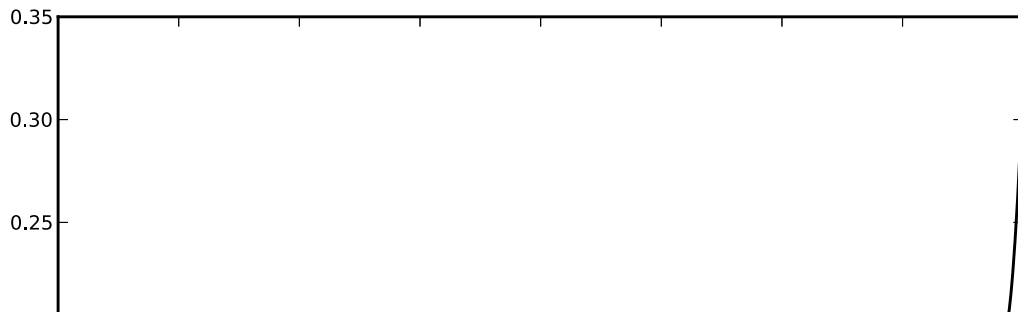

Here, we see that the frames are exactly equal at -3075, and the modes are much more nearly equal than they were initially.

On the other hand, aligning at one instant may not be satisfactory. Comparing the plots of  $|\vec{\omega}|$  above, we see that the secular angular frequencies don't seem to match, even though the instantaneous ones do. We might want to "smooth out" the cyclical changes by minimizing the difference over a region. In particular, we add a constant time offset  $\delta t$  and a constant rotation offset  $R_\delta$  to minimize

$$\int_{t_1}^{t_2} 4 |R_A(t) \bar{R}_B(t + \delta t) \bar{R}_\delta|^2 dt$$

Choosing  $t_1$  and  $t_2$  to lie around -3075, for example:

```

In [38]: # Align over a region
W_A.AlignTimeAndFrame(W_B, -3500, -2500);

# Show the differences
W_diff = W_A.Compare(W_B)
figure()
for m in range(-2,2+1) : plot(W_diff.T(), W_diff.Re(W_diff.FindModeIndex(2,m)), label=r'$m={0}$'.
ylabel(r"""\Delta \operatorname{Re}\{r\}, h^{2,m}/M\, \}""");
xlabel(r"$ (t-t_{\mathrm{merger}})/M$");
legend();
figure()
plot(W_diff.T(), [r.angle() for r in W_diff.Frame()]);
ylabel(r"""\Phi_{\Delta} (radians)""");
xlabel(r"$ (t-t_{\mathrm{merger}})/M$");

```

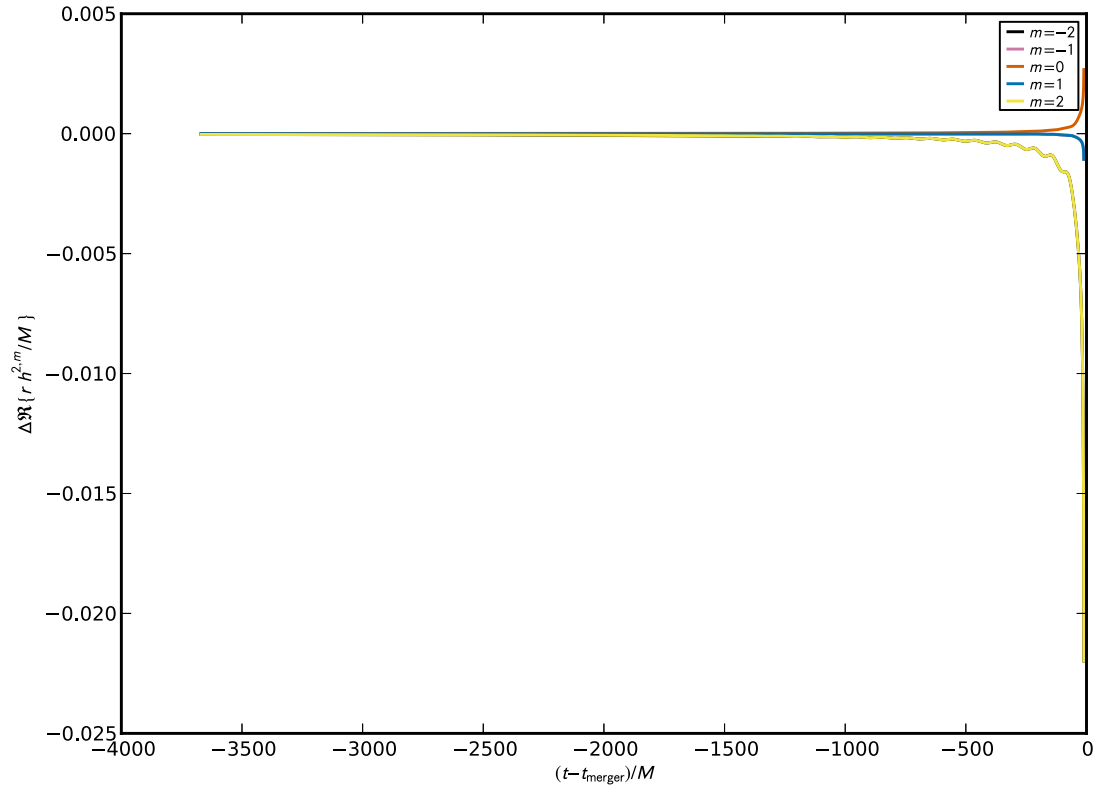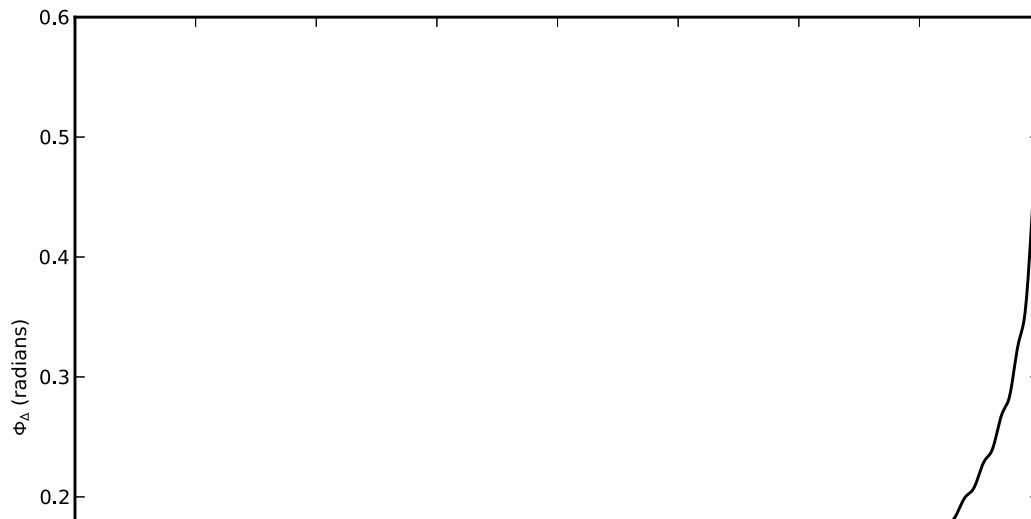

We see that the mode differences are essentially the same, but the frames are aligned more closely over a broader range of time.

## Appendix A: Quaternions and rotations

### Appendix A 1: Elements of quaternion mathematics

We create a Quaternion with components (1,2,3,5) as:

```
In [7]: Q = GWFrames.Quaternion(1,2,3,5) # These components are just randomly made up as an example
```

Its conjugate is

```
In [8]: Q.conjugate()
```

```
Out[8]: Quaternion(1.0, -2.0, -3.0, -5.0)
```

We can multiply by another quaternion:

```
In [9]: Q2 = GWFrames.Quaternion(7,11,13,17) # Also randomly made-up components
Q*Q2
```

```
Out[9]: Quaternion(-139.0, 11.0, 55.0, 45.0)
```

Notice that the product is *not* commutative in general:

```
In [10]: Q2*Q # This result is not the same as the last result
```

```
Out[10]: Quaternion(-139.0, 39.0, 13.0,
59.0)
```

The norm of a quaternion is given by

```
In [11]: sqrt( Q * Q.conjugate() )
```

```
Out[11]: Quaternion(6.244997998398398, 0.0, 0.0,
0.0)
```

or, equivalently

```
In [12]: Q.abs()
```

```
Out[12]: 6.244997998398398
```

The inverse of a quaternion is given by

```
In [13]: Qinv = Q.conjugate() / Q.normsquared()
Q * Qinv # We might get some roundoff garbage, but this is basically 1
```

```
Out[13]: Quaternion(1.0, 5.551115123125783e-17, 0.0,
0.0)
```



We can normalize a quaternion and obtain unit quaternion (which is a rotor):

```
In [14]: R = Q.normalized()
         R.abs()
```

```
Out[14]: 1.0
```

Ordinary vectors are just quaternions with 0 scalar part:

```
In [15]: x = GWFrames.Quaternion(0,1,0,0)
         y = GWFrames.Quaternion(0,0,1,0)
         z = GWFrames.Quaternion(0,0,0,1)
```

This allows us to define a rotor by its axis-angle description. The following uses the quaternion exponential function to give us a rotation about the  $x$  axis through the angle  $\pi/2$ :

```
In [16]: theta = pi/2.
         R = GWFrames.exp(theta * x / 2)
         R
```

```
Out[16]: Quaternion(0.7071067811865476, 0.7071067811865475, 0.0,
                  0.0)
```

So, for example, we can rotate  $y$  to get  $z$  (within numerical precision):

```
In [17]: R * y * R.conjugate()
```

```
Out[17]: Quaternion(0.0, 0.0, 2.220446049250313e-16,
                  1.0)
```

Or  $z$  to get  $-y$ :

```
In [18]: R * z * R.conjugate()
```

```
Out[18]: Quaternion(0.0, 0.0, -1.0,
                  2.220446049250313e-16)
```

We also have a convenient way to calculate the logarithm of a quaternion. For our rotor above, we get

```
In [19]: R.log()
```

```
Out[19]: Quaternion(0.0, 0.7853981633974482, 0.0,
                  0.0)
```

In this case, we get the correct inverse. However, note that in general we have branch-cut discontinuities as in the case of the usual complex logarithm. For example, the following exponential gives the same rotor as  $R$  above:

```
In [24]: GWFrames.exp(theta*x/2 + 2*pi*x)
```

```
Out[24]: Quaternion(0.7071067811865477, 0.7071067811865474, 0.0,
                  0.0)
```

## Appendix A 2: Formulas for rotations of SWSHs

Though they may not be directly useful for our purposes, this module includes implementations of the Wigner  $\mathcal{D}$  matrices and the

spin-weighted spherical harmonics in terms of quaternions directly, with no transformations to Euler angles or other representations.

```
In [62]: R = GWFrames.exp(pi * GWFrames.Quaternion(0,1,0,0) / 4) # Rotate by pi/2 about x
D = GWFrames.WignerDMatrix()
D.SetRotation(R)
D(2,1,-1) # Evaluate the ell=2, m'=1, m=-1 component of the Wigner D matrix with the rotation set
```

```
Out[62]: (-0.5000000000000001+0j)
```

```
In [65]: s = -2 # The spin weight
Ra = GWFrames.Quaternion(pi/2,pi/2) # Rotor corresponding to (vartheta, varphi) = (pi/2,pi/2)
Ylm = GWFrames.SWSH(s, Ra)
[Ylm(2,m) for m in [-2,-1,0,-1,2]]
```

```
Out[65]: [(-0.15769578262625994-7.003099550318303e-17j),
(7.003099550318305e-17-0.31539156525252j),
(0.3862742020231896+3.1100009458021847e-32j),
(7.003099550318305e-17-0.31539156525252j),
(-0.1576957826262601+7.003099550318306e-17j)]
```

For functions that actually implement rotations on waveform objects, see Appendix B below.

## Appendix A 3: Integrating the angular velocity

Though maybe not directly useful, a function that is used many places throughout the code is the one that takes the angular-velocity vector as a function of time, and integrates to find the frame with that velocity. For example, in the function `GWFrames.TransformToCorotatingFrame`, the following frame is used:

```
In [ ]: R_corot = GWFrames.FrameFromAngularVelocity(GWFrames.Quaternions(W_PN.AngularVelocityVector()), W_PN)
```

## Appendix A 4: Interpolation

It is important to be able to smoothly interpolate rotations. Here, we construct a series of 5 rotors, along with their respective time steps, and interpolate them to a finer series. Here, we plot the north pole as rotated by the various rotors. The original 5 points are plotted as large green circles, and the interpolated data is plotted as small red circles. We see that the interpolated data is very nicely smoothed.

```

In [39]: import GWFrames
from mpl_toolkits.mplot3d import Axes3D

# Define the basis vectors
x = GWFrames.Quaternion(0,1,0,0)
y = GWFrames.Quaternion(0,0,1,0)
z = GWFrames.Quaternion(0,0,0,1)

# Define some sparse input data to be interpolated
qIn = [GWFrames.exp((0./2.0)*(x)).normalized(),
        GWFrames.exp((math.pi/2./2.0)*(x)).normalized(),
        GWFrames.exp((math.pi/2./2.0)*(x+y)).normalized(),
        GWFrames.exp((math.pi/2./2.0)*(y)).normalized(),
        GWFrames.exp((8*math.pi/20./2.0)*(x+y)).normalized())
]
tIn = [-10.0, 5.0, 10.0, 15.0, 20.0]

# Interpolate the data to much finer steps
NSteps = 80
tOut = linspace(tIn[0], tIn[-1], NSteps)
qOut = GWFrames.Squad(qIn, tIn, tOut)

# Visualize in 3-D
vartheta = linspace(0, pi, 100)
varphi = linspace(0, 2 * pi, 100)
Sphere_x = outer(sin(vartheta), cos(varphi))
Sphere_y = outer(sin(vartheta), sin(varphi))
Sphere_z = outer(cos(vartheta), ones_like(varphi))
QuatXYZIn = array([(R*z*R.conjugate()).vec() for R in qIn])
QuatXYZOut = array([(R*z*R.conjugate()).vec() for R in qOut])
fig = plt.figure()
ax = fig.add_subplot(111, projection='3d')
Surface = ax.plot_surface(0.95*Sphere_x, 0.95*Sphere_y, 0.95*Sphere_z,
                          rstride=5, cstride=5, linewidth=0.5, antialiased=False)
Dots1 = ax.plot(QuatXYZIn[:,0], QuatXYZIn[:,1], QuatXYZIn[:,2], 'go', ms=5)
Dots2 = ax.plot(QuatXYZOut[:,0], QuatXYZOut[:,1], QuatXYZOut[:,2], 'ro', ms=3)

```

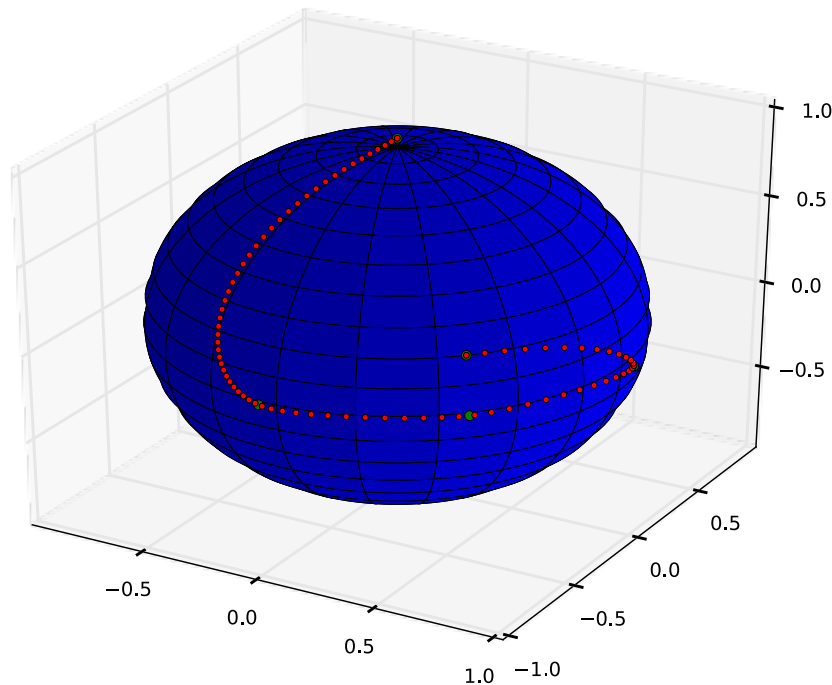

## Appendix B: Rotating spin-weighted functions

The previously discussed methods `TransformToSchmidtEtAlFrame`, `TransformToOShaughnessyEtAlFrame`, `TransformToAngularVelocityFrame`, `TransformToCorotatingFrame`, and `TransformToInertialFrame` are probably the most useful for transforming waveform objects into the appropriate frames. However, in general, we also have the method `RotateDecompositionBasis`, which takes an explicit rotor or array of rotors, and rotates the basis in which the waveform is decomposed. For example:

```
In [ ]: W_C = GWFrames.PNWaveform(W_PN)
        W_C.RotateDecompositionBasis(R_corot)
```

## Appendix C: Other methods of choosing a frame

### Appendix C 1: Maximization

```
In [ ]: # Make copy to transform. Because Python makes copies by reference,
        # to make a real copy, we need to use the copy constructor:
        W_PN_Aligned = GWFrames.PNWaveform(W_PN)

        # Now, transform the copy to the aligned frame
        W_PN_Aligned.TransformToSchmidtEtAlFrame()

        # And plot the waveform in the aligned frame
        ell=2
        ModeIndices = [W_PN.FindModeIndex(ell,m) for m in range(-ell,ell+1)]
        plt.figure(1)
        plt.subplot(121)
        for ModeIndex in ModeIndices : plt.plot(W_PN_Aligned.T(), W_PN_Aligned.Abs(ModeIndex))
        ylabel(r"$|r\, h^{2,m}/M\, |$");
        xlabel(r"$t-t_{\mathrm{merger}}/M$");
        plt.subplot(122)
        for ModeIndex in ModeIndices : plt.plot(W_PN_Aligned.T(), W_PN_Aligned.ArgUnwrapped(ModeIndex))
        ylabel(r"$\phi^{2,m}$ (radians)");
        xlabel(r"$t-t_{\mathrm{merger}}/M$");
```

### Appendix C 2: Dominant principal axis

```
In [ ]: # Make copy to transform. Because Python makes copies by reference,
# to make a real copy, we need to use the copy constructor:
W_PN_Aligned = GWFrames.PNWaveform(W_PN)

# Now, transform the copy to the aligned frame
W_PN_Aligned.TransformToOShaughnessyEtAlFrame()

# And plot the waveform in the aligned frame
ell=2
ModeIndices = [W_PN.FindModeIndex(ell,m) for m in range(-ell,ell+1)]
plt.figure(1)
plt.subplot(121)
for ModeIndex in ModeIndices : plt.plot(W_PN_Aligned.T(), W_PN_Aligned.Abs(ModeIndex))
ylabel(r"$|r\, h^2{}_m/M\, |$");
xlabel(r"$t-t_{\mathrm{merger}}/M$");
plt.subplot(122)
for ModeIndex in ModeIndices : plt.plot(W_PN_Aligned.T(), W_PN_Aligned.ArgUnwrapped(ModeIndex))
ylabel(r"$\phi^2{}_m$ (radians)");
xlabel(r"$t-t_{\mathrm{merger}}/M$");
```

### Appendix C 3: Aligned with the angular velocity

```
In [ ]: # Make copy to transform. Because Python makes copies by reference,
# to make a real copy, we need to use the copy constructor:
W_PN_Aligned = GWFrames.PNWaveform(W_PN)

# Now, transform the copy to the aligned frame
W_PN_Aligned.TransformToAngularVelocityFrame()

# And plot the waveform in the aligned frame
ell=2
ModeIndices = [W_PN.FindModeIndex(ell,m) for m in range(-ell,ell+1)]
plt.figure(1)
plt.subplot(121)
for ModeIndex in ModeIndices : plt.plot(W_PN_Aligned.T(), W_PN_Aligned.Abs(ModeIndex))
ylabel(r"$|r\, h^2{}_m/M\, |$");
xlabel(r"$t-t_{\mathrm{merger}}/M$");
plt.subplot(122)
for ModeIndex in ModeIndices : plt.plot(W_PN_Aligned.T(), W_PN_Aligned.ArgUnwrapped(ModeIndex))
ylabel(r"$\phi^2{}_m$ (radians)");
xlabel(r"$t-t_{\mathrm{merger}}/M$");
```

### Appendix C 4: The minimal-rotation condition

Each of the methods implemented above is applied with the minimal-rotation condition. But it may occasionally be useful in its own right.

```
In [ ]: ROut = GWFrames.MinimalRotation(RIn, TIn)
```
